# Supplementary material for: WaveFuzz: A Clean-Label Poisoning Attack to Protect Your Voice
Source: arXiv:2203.13497 source file (2022-03-25)
Supplement: Supplementary file 1 [file appendix.tex]

\appendix

\begin{figure*}[!t]
	\centering
	\subfigure[]{
		\begin{minipage}[b]{0.23\textwidth}
			\includegraphics[width=1.2\textwidth]{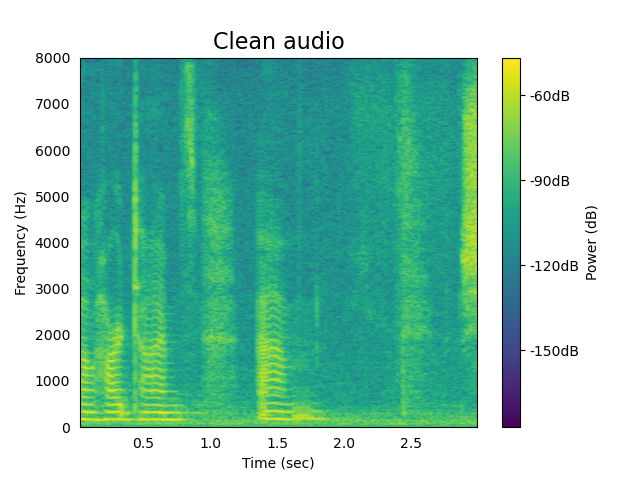}\\%
			
			\includegraphics[width=1.2\textwidth]{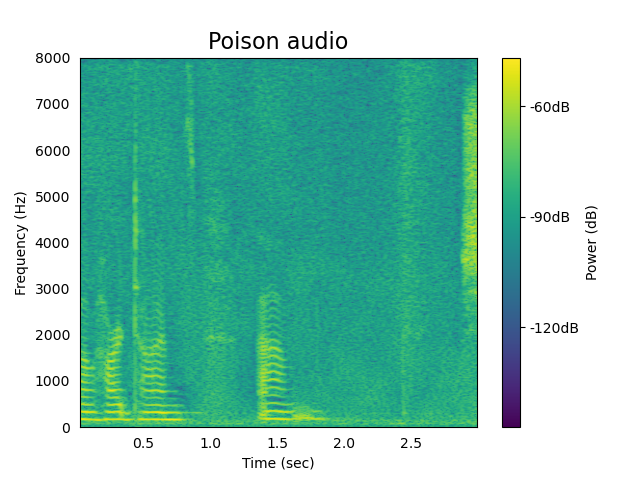}\\%
			
		\end{minipage}
	}
		\subfigure[]{
		\begin{minipage}[b]{0.23\textwidth}
				\includegraphics[width=1.2\textwidth]{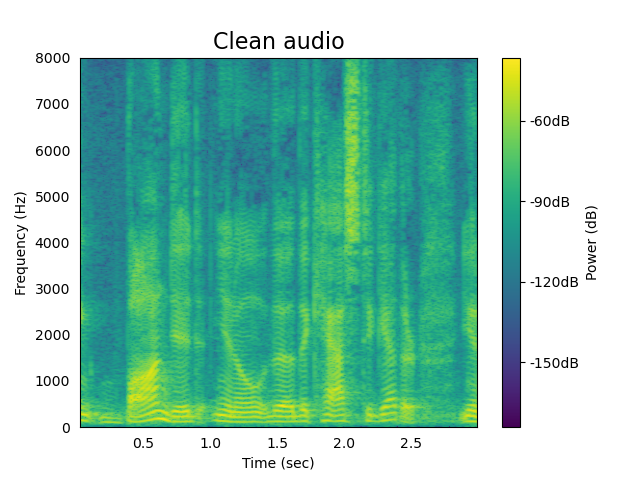}\\%
			
			\includegraphics[width=1.2\textwidth]{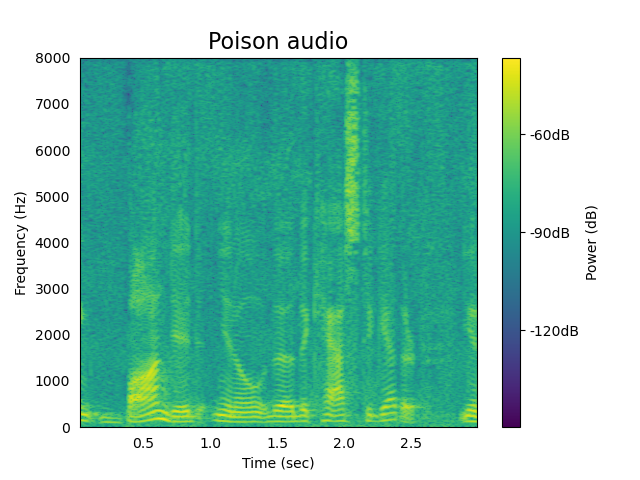}\\%
			
		\end{minipage}
	}
		\subfigure[]{
		\begin{minipage}[b]{0.23\textwidth}
				\includegraphics[width=1.2\textwidth]{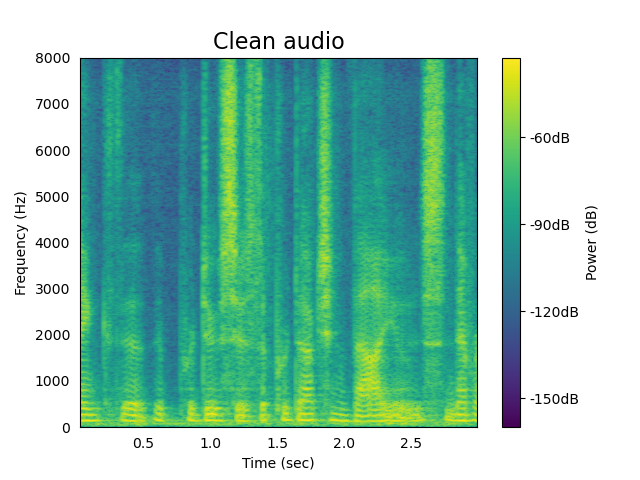}\\%
			
			\includegraphics[width=1.2\textwidth]{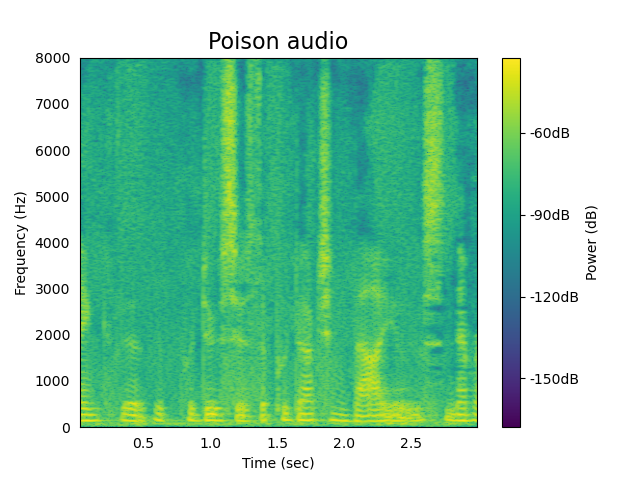}\\%
			
		\end{minipage}
	}
		\subfigure[]{
		\begin{minipage}[b]{0.23\textwidth}
				\includegraphics[width=1.2\textwidth]{fig/clean_3.png}\\%
			
			\includegraphics[width=1.2\textwidth]{fig/poison_3.png}\\%
			
		\end{minipage}
	}

	\caption{Spectrograms of benign audio and poisoned audio examples generated by our WaveFuzz. The top line images are spectrogram of benign examples, and the bottom line images are spectrogram of poisoned examples.}\label{SP}
\end{figure*}
\section{More  results}
three are more visualization results about spectrogram and wave. Moreover,  we experiment with each audio task to find the $\alpha$, where the results are in Table~\ref{TA:AL}. We select the $\alpha$, which obtains the current optimal performance to generate corrupted samples in our experiments.  

\begin{table}[t]
\centering

\begin{tabular}{ccccc} 
\toprule
       & \multicolumn{3}{c}{DAcc.(\%)}   & \multirow{2}{*}{PR(\%)}                       \\ 
\cmidrule{2-4}
$\alpha$   & 0.1     & 0.01    & 0.001   &                                           \\ 
\midrule
VggVox    & 24.55 & 21.69 & 21.66 & \multicolumn{1}{l}
{\multirow{2}{*}{5}}  \\
CNN & 9.75  & 7.75  & 6.75  & \multicolumn{1}{l}{}                      \\
\bottomrule
\end{tabular}
\caption{The selection of $\alpha$. }\label{TA:AL}
\end{table}
